# Supplementary material for: DreaMo: Articulated 3D Reconstruction From A Single Casual Video
Source: arXiv:2312.02617 source file (2023-12-07)
Supplement: Supplementary file 1 [file 6_suppl.tex]

\appendix

\begin{figure*}[ht!]
\begin{center}
\includegraphics[width=\textwidth]{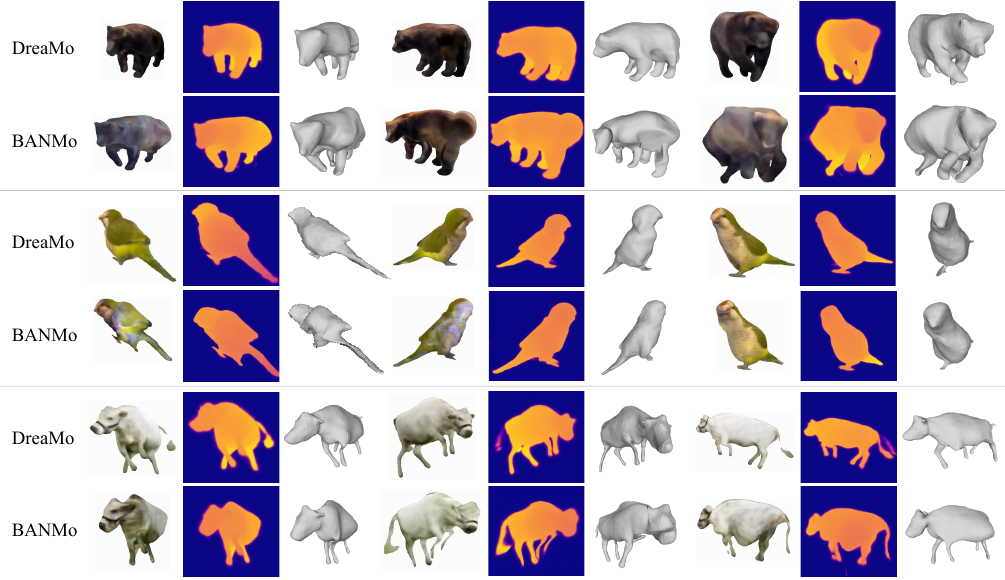}
\end{center}
\vspace{-1em}
\caption{
  \textbf{3D reconstruction comparison among BANMo~\cite{yang2022banmo} and our {\ourmethod}.}
  We show three rendered novel-view images, including RGB and depth, and their corresponding reconstructed shapes for each method.
}
\label{fig:suppl_reconst_results}
\end{figure*}

%%%%%%%%%%%%%%%%%%%%%%%%%%%%%%%%%%%%%%%%%%%%%%%%%%%%%%%%%%%%%%%%%%%%%%%%%%%%%%%%%%%%%%%%%%
\section{Supplementary Video}
Please watch the supplementary demo video for a comprehensive comparison between our method {\ourmethod} and the current state-of-the-art method BANMo~\cite{yang2022banmo}.
The video includes qualitative results of \Cref{sec:suppl-more-3d-reconst} and \Cref{sec:suppl-more-articulation} for novel view synthesis, 3D shape reconstruction, and novel pose articulation.

%%%%%%%%%%%%%%%%%%%%%%%%%%%%%%%%%%%%%%%%%%%%%%%%%%%%%%%%%%%%%%%%%%%%%%%%%%%%%%%%%%%%%%%%%%

\section{More Results for 3D Reconstruction}
\label{sec:suppl-more-3d-reconst}
We provide more 3D reconstruction results in \Cref{fig:suppl_reconst_results} to compare between BANMo~\cite{yang2022banmo} and our proposed {\ourmethod}.
The figure shows that BANMo produces texture artifacts and irregular shapes due to insufficient view coverage.
In contrast, benefiting from simultaneously reconstructing training-view frames and hallucinating unobserved regions of the target subjects, {\ourmethod} generates more plausible rendered images and convincing shapes.

%%%%%%%%%%%%%%%%%%%%%%%%%%%%%%%%%%%%%%%%%%%%%%%%%%%%%%%%%%%%%%%%%%%%%%%%%%%%%%%%%%%%%%%%%%
\section{More Results for Articulating 3D Model}
\label{sec:suppl-more-articulation}
\begin{figure*}[ht!]
\begin{center}
\includegraphics[width=\textwidth]{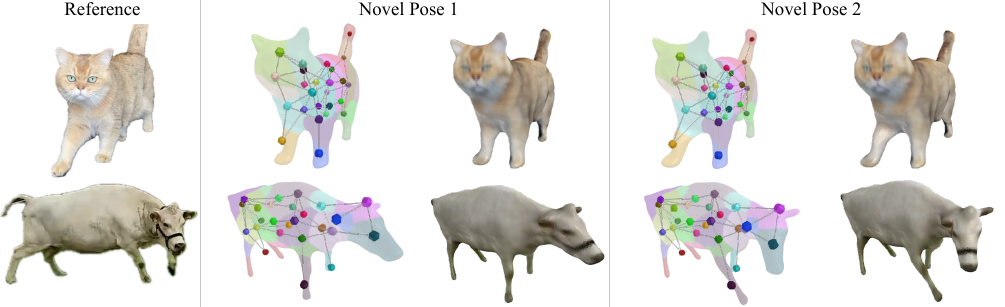}
\end{center}
\vspace{-1.5em}
\caption{
  \textbf{Manipulating {\ourmethod} by controlling the generated skeletons.}
  We manually modify the bone positions and warp the associated skin to manipulate the reconstructed model into new poses.
}
\label{fig:suppl_articulate_model}
\end{figure*}

\begin{figure*}[ht]
\begin{center}
\includegraphics[width=\textwidth]{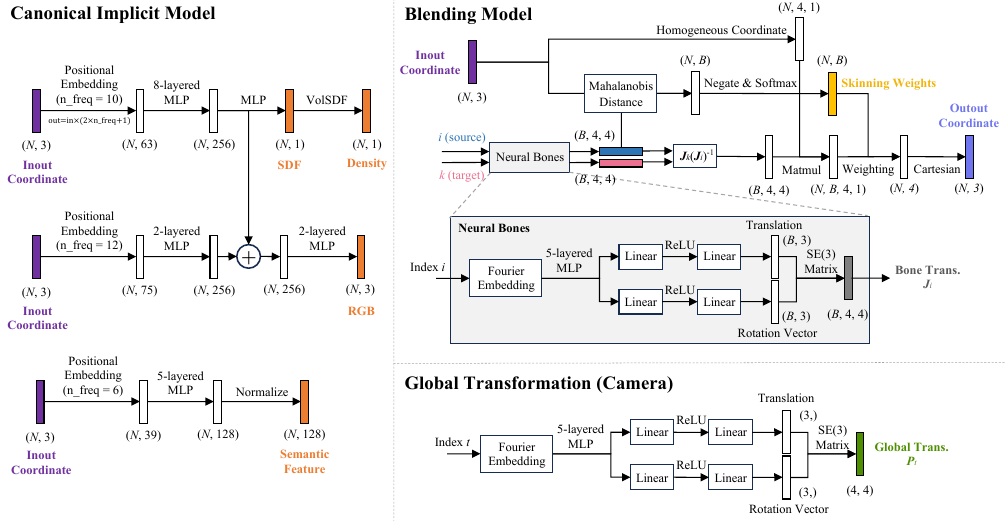}
\end{center}
\vspace{-1.5em}
\caption{
  \textbf{Network architecture of {\ourmethod}.}
  We present the network design of the canonical implicit model (left), the blending models (upper right), and the global transformation model (lower right).
  The warping models, which transform 3D coordinates between canonical and observation spaces, integrate blending and global transformation models, as elaborated in Section 3.1.
}
\label{fig:suppl_network_arch}
\end{figure*}

In \Cref{fig:suppl_articulate_model}, we provide more examples for controlling {\ourmethod}.
Following the 3D model manipulation described in Section 3.1, we manually control the generated skeleton and transform the skin points (\ie vertices of the mesh) to produce novel poses.
With the accurately learned bone placement, skinning weights, and 3D shapes from {\ourmethod}, the skin points can be reasonably transitioned in response to the movement of the neural bones.
This results in realistic outcomes for novel poses.

%%%%%%%%%%%%%%%%%%%%%%%%%%%%%%%%%%%%%%%%%%%%%%%%%%%%%%%%%%%%%%%%%%%%%%%%%%%%%%%%%%%%%%%%%%
\section{Implementation Details}
\subsection{Network Architecture}
\label{sec:suppl-network-arch}
In \Cref{fig:suppl_network_arch}, we show the network architecture of the canonical implicit model, the blending model, and the global transformation model.

Similar to BANMo~\cite{yang2022banmo}, we use MLPs for the canonical implicit model, where different frequencies for the positional embedding are employed to model the various degrees of change for density, appearance, and semantic features.
Following VolSDF~\cite{yariv2021volsdf}, the SDF values can be converted to density by the cumulative distribution function of the Laplacian distribution.

The blending model transforms a given input coordinate into the output coordinate based on the subject's deformation, which the skinning weights and the transformation between the source and target bones can determine.
Specifically, the skinning weights are calculated based on the Mahalanobis distance between the input coordinates and the source neural bones.
This distance is then negated and normalized by a subsequent softmax layer.
On the other hand, the bone positions for each time step can be acquired using frame-wise Fourier embedding~\cite{yang2022banmo, mildenhall2021nerf}, followed by an MLP.

Finally, the global transformation, representing the camera transformation, is obtained by feeding the frame-wise Fourier embedding into the subsequent MLP.

\subsection{3D Shape Reconstruction}
\label{sec:suppl-shape-reconst}
We perform two steps to reconstruct the subject's shape in a specific video frame.
First, using marching cubes, we extract the rest-pose mesh, which represents the 3D shape of the reconstructed subject, from the neural implicit model in canonical space.
Afterward, we apply the forward warping model to transform each vertex on the mesh to the observation space at the time step of the given video frame.

%%%%%%%%%%%%%%%%%%%%%%%%%%%%%%%%%%%%%%%%%%%%%%%%%%%%%%%%%%%%%%%%%%%%%%%%%%%%%%%%%%%%%%%%%%
\section{Dataset}
\label{sec:dataset}
We show the diverse species in the self-collected dataset in \Cref{fig:suppl_dataset}.
It is important to note that the images in \Cref{fig:suppl_dataset} have been cropped just for visualization.
This cropping does not imply that the target subjects in the training video are large and centered.

\begin{figure}[ht!]
\begin{center}
\includegraphics[width=.92\linewidth]{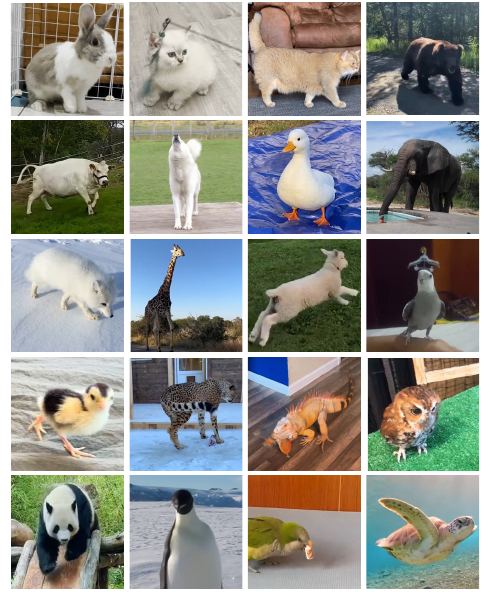}
\end{center}
\vspace{-1.2em}
\caption{
  Our self-collected video dataset for diverse species and insufficient view coverage from the Internet.
  We present some cropped images from the entire dataset.
}
\label{fig:suppl_dataset}
\end{figure}
