# Supplementary material for: DreaMo: Articulated 3D Reconstruction From A Single Casual Video
Source: arXiv:2312.02617 source file (2023-12-07)
Supplement: Supplementary file 2 [file suppl_articulate_model.tex]

\begin{figure*}[ht!]
\begin{center}
\includegraphics[width=\textwidth]{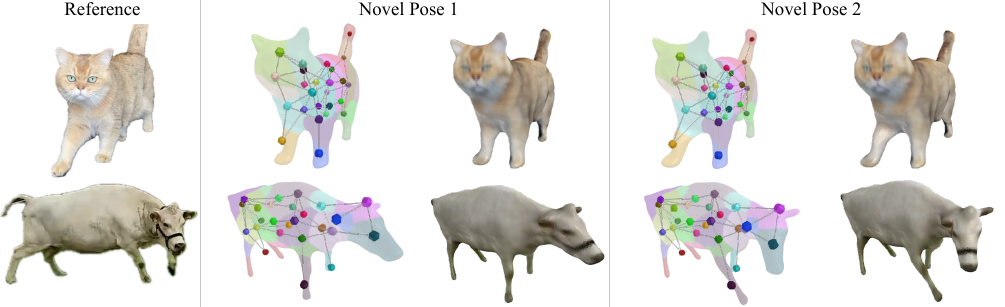}
\end{center}
\vspace{-1.5em}
\caption{
  \textbf{Manipulating {\ourmethod} by controlling the generated skeletons.}
  We manually modify the bone positions and warp the associated skin to manipulate the reconstructed model into new poses.
}
\label{fig:suppl_articulate_model}
\end{figure*}
