# Supplementary material for: DreaMo: Articulated 3D Reconstruction From A Single Casual Video
Source: arXiv:2312.02617 source file (2023-12-07)
Supplement: Supplementary file 3 [file suppl_dataset.tex]

\begin{figure}[ht!]
\begin{center}
\includegraphics[width=.92\linewidth]{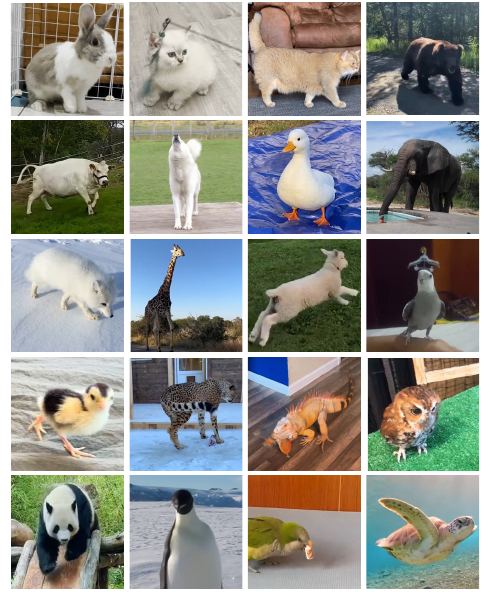}
\end{center}
\vspace{-1.2em}
\caption{
  Our self-collected video dataset for diverse species and insufficient view coverage from the Internet.
  We present some cropped images from the entire dataset.
}
\label{fig:suppl_dataset}
\end{figure}
