# Supplementary material for: DreaMo: Articulated 3D Reconstruction From A Single Casual Video
Source: arXiv:2312.02617 source file (2023-12-07)
Supplement: Supplementary file 4 [file suppl_network_arch.tex]

\begin{figure*}[ht]
\begin{center}
\includegraphics[width=\textwidth]{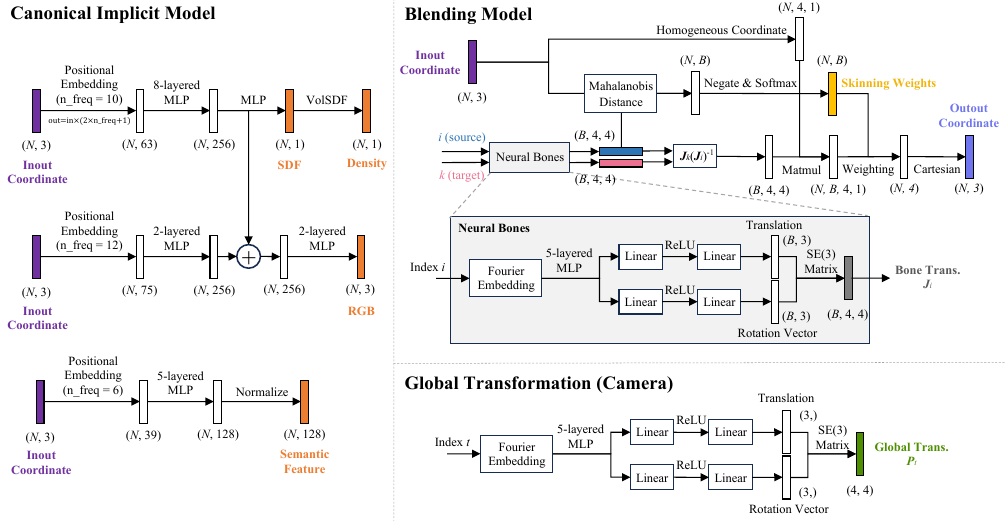}
\end{center}
\vspace{-1.5em}
\caption{
  \textbf{Network architecture of {\ourmethod}.}
  We present the network design of the canonical implicit model (left), the blending models (upper right), and the global transformation model (lower right).
  The warping models, which transform 3D coordinates between canonical and observation spaces, integrate blending and global transformation models, as elaborated in Section 3.1.
}
\label{fig:suppl_network_arch}
\end{figure*}
