# Supplementary material for: DreaMo: Articulated 3D Reconstruction From A Single Casual Video
Source: arXiv:2312.02617 source file (2023-12-07)
Supplement: Supplementary file 5 [file suppl_reconst_results.tex]

\begin{figure*}[ht!]
\begin{center}
\includegraphics[width=\textwidth]{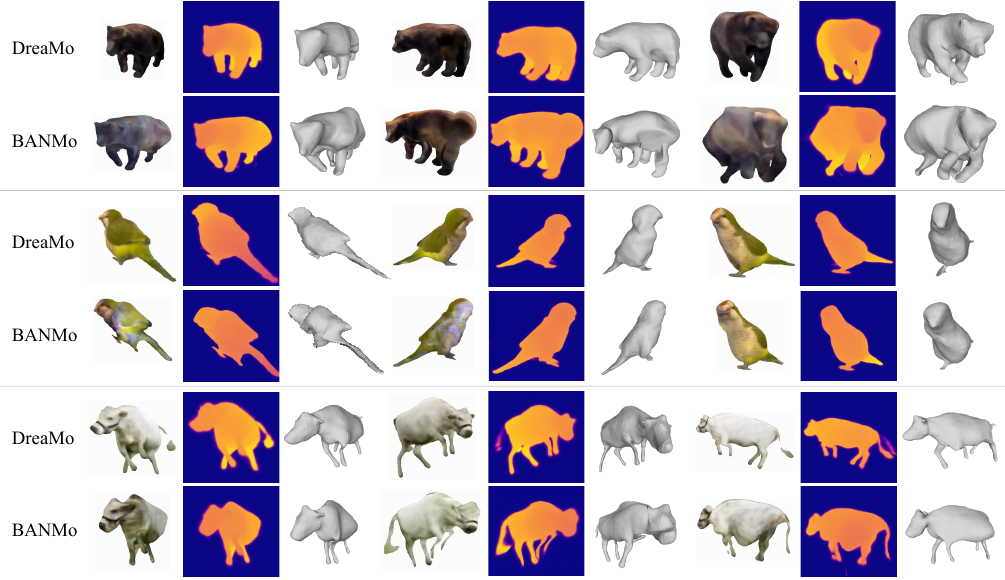}
\end{center}
\vspace{-1em}
\caption{
  \textbf{3D reconstruction comparison among BANMo~\cite{yang2022banmo} and our {\ourmethod}.}
  We show three rendered novel-view images, including RGB and depth, and their corresponding reconstructed shapes for each method.
}
\label{fig:suppl_reconst_results}
\end{figure*}
